# Supplementary material for: Thermodynamically consistent machine learning model for excess Gibbs energy
Source: arXiv:2509.06484 ancillary file (2026-02-20)
Supplement: Supplementary file 1 [file supporting_information.pdf]

---

# SUPPORTING INFORMATION FOR A MACHINE-LEARNED EXPRESSION FOR THE EXCESS GIBBS ENERGY

---

**Marco Hoffmann<sup>†</sup>**

Laboratory of Engineering Thermodynamics  
RPTU Kaiserslautern, Germany  
marco.hoffmann@rptu.de

**Thomas Specht<sup>†</sup>**

Laboratory of Engineering Thermodynamics  
RPTU Kaiserslautern, Germany  
thomas.specht@rptu.de

**Quirin Göttl**

Laboratory of Chemical Process Engineering  
Technical University of Munich, Germany  
qgctvtum@gmail.com

**Jakob Burger**

Laboratory of Chemical Process Engineering  
Technical University of Munich, Germany  
burger@tum.de

**Stephan Mandt**

Department of Computer Science & Statistics  
University of California, Irvine  
mandt@uci.edu

**Hans Hasse**

Laboratory of Engineering Thermodynamics  
RPTU Kaiserslautern, Germany  
hans.hasse@rptu.de

**Fabian Jirasek\***

Laboratory of Engineering Thermodynamics  
RPTU Kaiserslautern, Germany  
fabian.jirasek@rptu.de

## 1 Data curation of activity coefficients at infinite dilution in mixed solvents

During data preprocessing, we observed that some ACI data for ternary mixtures (i.e., in mixed solvents) in the DDB were incorrect, as the labels of the two solvents had been interchanged. We therefore applied the following curation protocol for all ternary ACI data before including them in our data set:

For each ternary ACI data point given for temperature  $T_{\text{ACI}}$ , we first verified that experimental data for infinite dilution activity coefficients of the same solute are available in both *pure* solvents in the binary ACI database at temperatures within  $\pm 5$  K of  $T_{\text{ACI}}$ . All ternary ACI data points, for which this was not the case, were excluded. When the comparison indicated the solvents were in the wrong order, we swapped their order accordingly.

---

\*Corresponding author

<sup>†</sup>These authors contributed equally.

## 2 Surrogate solver

The surrogate solvers were trained individually for each fold on the corresponding LLE training data, specifically, synthetic data for the Gibbs energies of mixing for the systems and temperatures calculated with mod. UNIFAC. The surrogate solvers were trained for 200 epochs, using the Adam optimizer with the MSE loss and the OneCycleLR scheduler ( $\text{max\_lr}=0.01$ ), and the best model was selected based on the validation loss (the validation data set was obtained analog to the training set, as described in the manuscript). Over all folds and test systems we find that the phase compositions  $x'_i, x''_i$  are predicted with an average error of about 0.004, which is likely lower than the uncertainties of most experimental data points. In Fig. S.1 we provide an example of the functionality of the surrogate solver on a test system of the first fold, namely the system hexane + water. Fig. S.1 demonstrates that, for this system, the surrogate solver's predictions perfectly match the CEM's calculations and that the two methods can be used interchangeably.

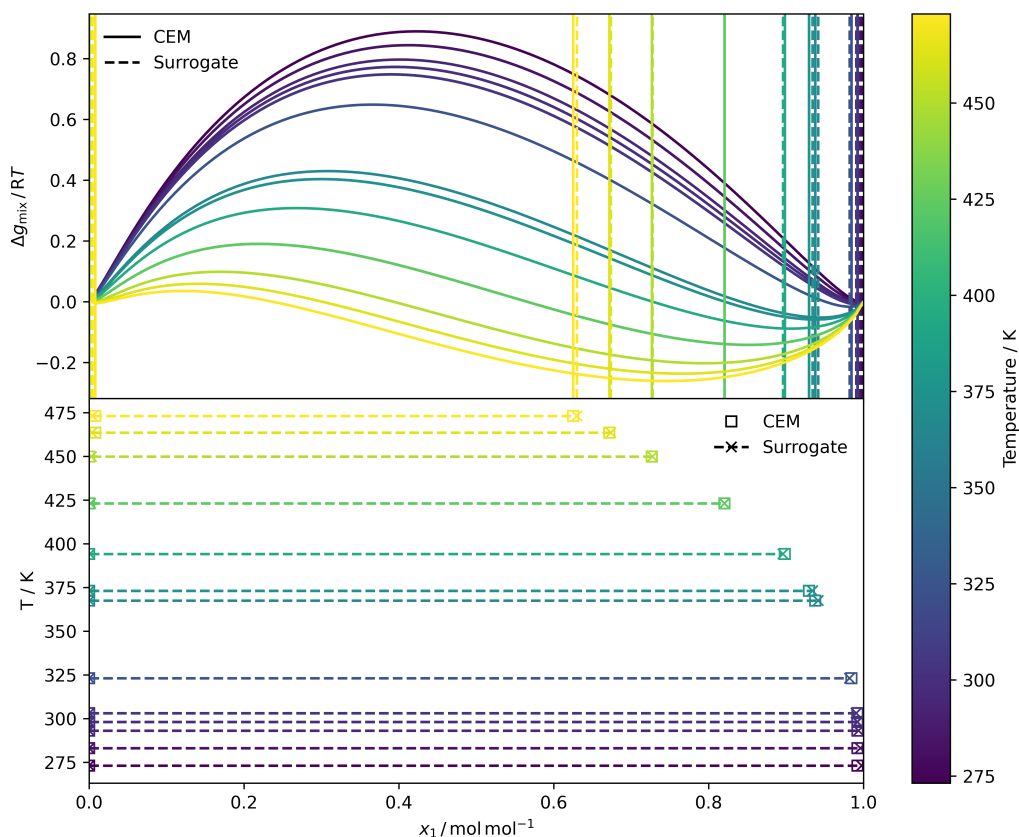

Figure S.1: Evaluation of the surrogate solver of fold one on the test system hexane (1) + water (2). Top: Gibbs energy of mixing  $\Delta g_{\text{mix}}/RT$  curves over the mole fraction  $x_1$  calculated from mod. UNIFAC for different temperatures. The vertical lines show the LLE phase compositions calculated by the CEM (solid) and predicted by the surrogate solver (dashed). Bottom: LLE phase diagram for the system obtained with the CEM and the surrogate solver. Colors in both diagrams correspond to the temperatures indicated by the color bar.

### 3 Grid search

The optimal hyperparameters of HANNA were determined using a grid search performed on the first fold. In this work, we only varied the weights of the LLE loss, the Gibbs loss, and the Lipschitz regularization term, cf. Eqs. (8), (10), (15) in the manuscript, but not additional hyperparameters of the HANNA architecture, such as the number of nodes per layer or the number of layers in the FFNNs, which were adopted from our prior work [1]. Tab. S.1 shows the search space and marks the hyperparameters of the selected model configuration. The search space also includes model variants that were trained without LLE data, the Gibbs loss, or the Lipschitz regularization (by setting the respective weights to zero) to assess their general impact on the model performance. To improve the robustness of the evaluation, for each hyperparameter setting, an ensemble of two models with different initial weights was trained to the training data of fold one and their predictions averaged. The hyperparameter selection was based on the error scores of the three different data types (VLE, ACI, LLE) on the validation set of fold one, as well as on the percentage of LLE systems for which the model correctly predicted a liquid-liquid phase split. Below, we discuss the impact of each hyperparameter in detail.

Table S.1: Hyperparameter search space used in the grid search. The hyperparameter values of the model configuration selected for training the final models are denoted in bold.

| Hyperparameter     | Search space                                                                       |
|--------------------|------------------------------------------------------------------------------------|
| $w_{\text{LLE}}$   | 0, 1.0, 5.0, <b>10.0</b>                                                           |
| $w_{\text{Lips}}$  | 0, $10^{-4}$ , $2 \cdot 10^{-4}$ , <b><math>5 \cdot 10^{-4}</math></b> , $10^{-3}$ |
| $w_{\text{Gibbs}}$ | 0, <b>0.001</b> , 0.005, 0.01, 0.05                                                |

**Impact of LLE training** Fig. S.2 shows how the training on LLE data impacts the model accuracy on the different data types. The scores on the VLE and ACI data on the validation set do not significantly change with varying LLE loss weights. However, the errors on the LLE data are greatly reduced, and the percentage of correctly predicted phase splits improves with increasing LLE loss weights. This proves that training on LLE data enables accurate predictions for unseen LLE systems, and more importantly, that the surrogate solver works as intended. Moreover, it is evident that HANNA can capture the non-ideal behavior of the fluid phase in both the VLE and LLE regimes simultaneously, and does not require two separate parameterizations, unlike many traditional methods. Based on the grid search result, we selected  $w_{\text{LLE}} = 10.0$  for the final model configuration.

**Impact of Gibbs loss** The purpose of the Gibbs loss is to force the model to produce correct  $\Delta g_{\text{mix}}$  curves that lead to a phase split for the LLE data in the training. The loss is only applied to the systems for which this is not the case (cf. Section "Training of HANNA" in the manuscript) and should therefore not have much impact on the other data types (VLE and ACI). Fig. S.3 confirms this assumption: only the percentage of systems with correctly identified phase splits increases significantly with increasing  $w_{\text{Gibbs}}$ , while no significant dependence of the other error scores from  $w_{\text{Gibbs}}$  is observed. The results demonstrate that incorporating the Gibbs loss into the training increases the number of LLE phase splits that HANNA can correctly predict, thereby expanding the model's applicability range. We noticed that while high values of  $w_{\text{Gibbs}}$  lead to a larger number of systems with a correctly predicted phase split, it also leads to two-phase regions that extend further than the experimentally measured upper and lower critical solution temperatures. This is likely because through this behavior the model can avoid a Gibbs loss. Consequently, we selected  $w_{\text{Gibbs}} = 0.001$  as a good compromise for the final model configuration.

**Impact of Lipschitz Regularization** The Lipschitz regularization controls the smoothness of the neural network output by encouraging a small Lipschitz constant. A higher regularization weight  $w_{\text{Lips}}$  promotes more smoothness but restricts the flexibility of the model. The ideal regularization weight should still provide the model with sufficient flexibility to extrapolate to unseen data. Fig. S.4 shows that the best  $w_{\text{Lips}}$  in the grid search is 0.0001. While the impact on the VLE loss appears negligible, the ACI loss varies significantly across the search space, and especially for values larger than 0.0001, the ACI loss increases substantially, presumably because the model's flexibility becomes too limited. While the error scores on the different data types give a good quantitative representation of the model accuracy for the considered phase equilibria, they do not contain direct information on the smoothness of the predictions. In fact, we found that for small values of  $w_{\text{Lips}}$ , the number of LLE systems with unphysical artifacts, such as sudden changes in phase compositions over temperature, increased. On the other hand, larger values of  $w_{\text{Lips}}$  led to a higher error on the ACI data. Since HANNA still outperforms the benchmarks on ACI data, even for higher values of  $w_{\text{Lips}}$ , we decided to prioritize model smoothness and robustness over accuracy on ACI data and therefore chose  $w_{\text{Lips}} = 0.0005$  for the final model configuration.

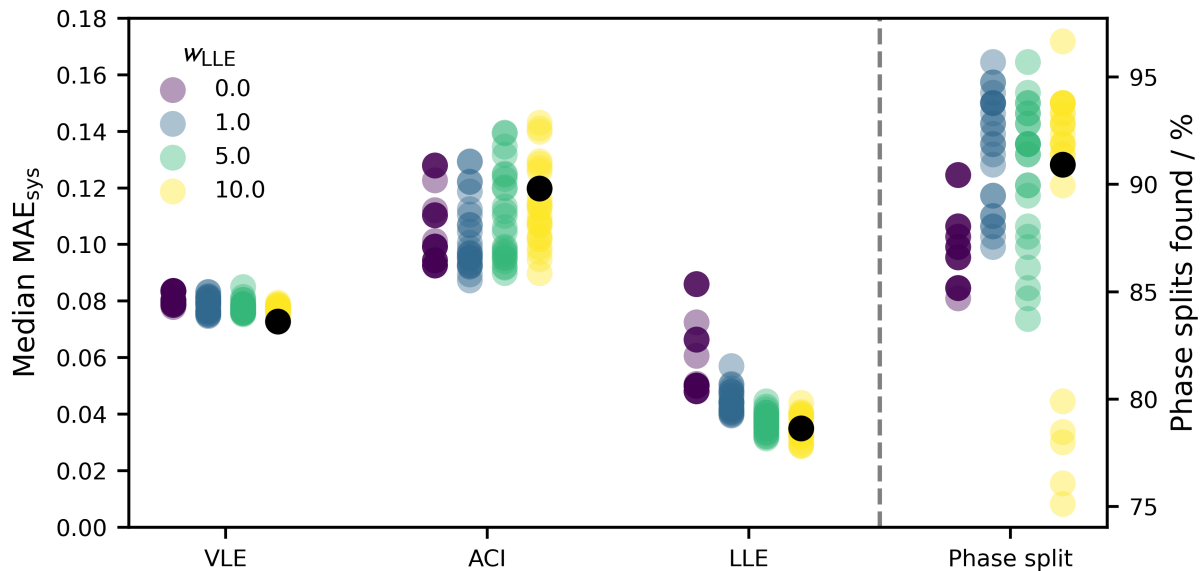

Figure S.2: Scatter plot visualizing the impact of different weights  $w_{LLE}$  of the LLE loss  $\mathcal{L}_{LLE}$  on the model accuracy on validation data for the three different data types. For each data type, all models of the grid search are colored and aligned by their  $w_{LLE}$  in the training. The group on the outer right shows the percentage of systems for which a liquid-liquid phase split is correctly predicted. The black markers denote the selected model configuration.

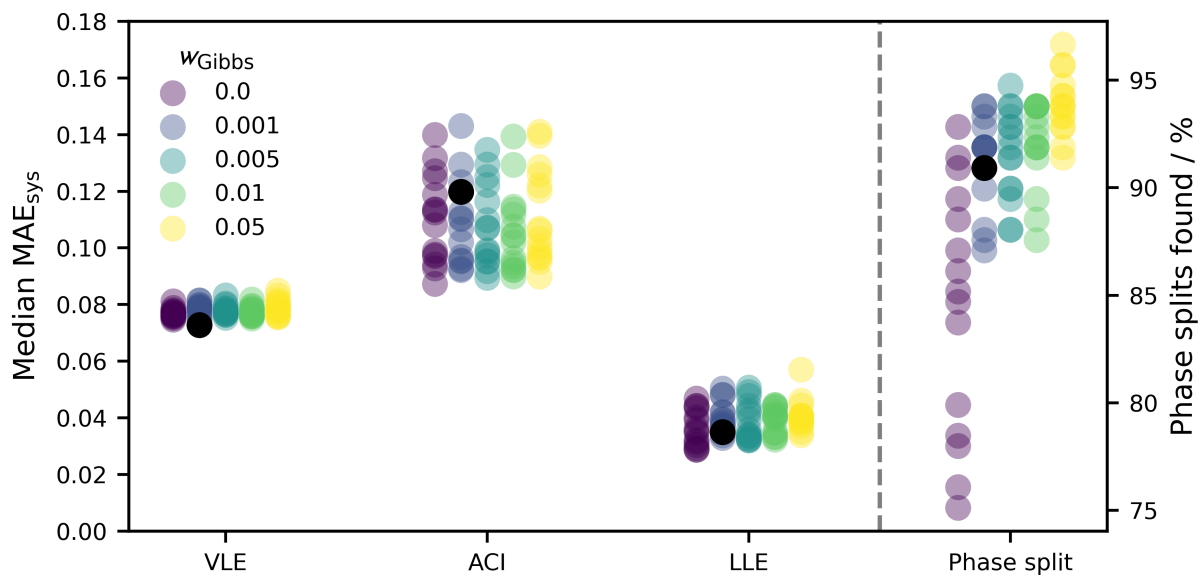

Figure S.3: Scatter plot visualizing the impact of different weights  $w_{Gibbs}$  of the Gibbs loss  $\mathcal{L}_{Gibbs}$  on the model accuracy on validation data for the three different data types. For each data type, all models of the grid search are colored and aligned by their consistency loss weight in the training. The group on the outer right shows the percentage of systems for which a liquid-liquid phase split is correctly predicted. Only model variants with LLE training ( $w_{LLE} > 0$ ) are shown. The black markers denote the selected model configuration.

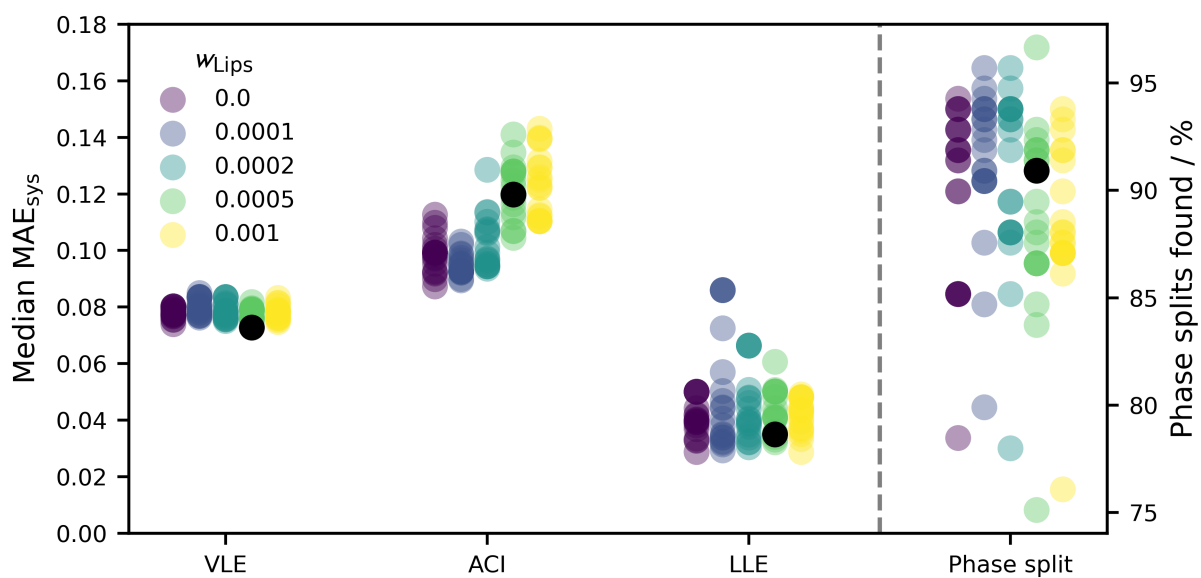

Figure S.4: Scatter plot visualizing the impact of different weights  $w_{\text{Lips}}$  of the Lipschitz regularization term  $\mathcal{L}_{\text{Lips}}$  on the model accuracy on validation data for the three different data types. For each data type, all models of the grid search are colored and aligned by their Lipschitz regularization weight in the training. The group on the outer right shows the percentage of systems for which a liquid-liquid phase split is correctly predicted. The black markers denote the selected model configuration.

## 4 Additional results

### 4.1 Binary phase equilibria with mod. UNIFAC

Fig. S.5 shows six phase equilibria predicted with HANNA and mod. UNIFAC. The systems correspond to those systems from Fig. 2b, 2c and 2d in the manuscript that are within the mod. UNIFAC horizon, i.e. two systems with VLE (top row, left and middle plot), one system with LLE (top row, right plot) and three heteroazeotropes (bottom row). Note that mod. UNIFAC was likely fitted to many of the presented systems here and the comparison is therefore biased towards mod. UNIFAC.

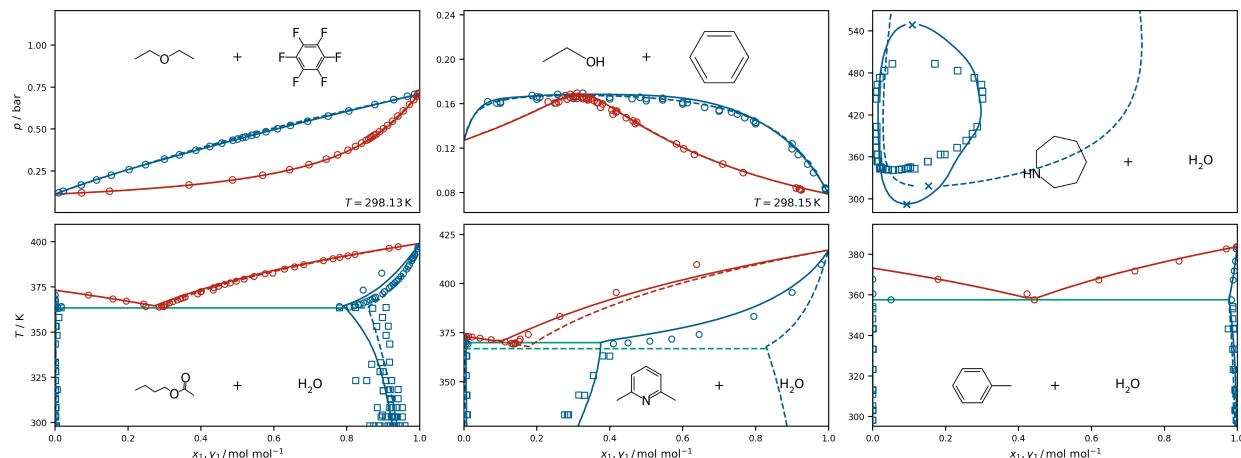

Figure S.5: Predicted phase equilibria with HANNA (solid lines) and mod. UNIFAC (dashed lines) for six binary systems. Open symbols mark experimental data. Blue color marks the liquid phase; red color marks the vapor phase. Molecular structures of the components are depicted within the plots. The left molecule corresponds to the first component.

### 4.2 Predictions for quaternary systems

Fig. S.6 compares the VLE and LLE predictions of HANNA for quaternary systems to those of mod. UNIFAC. For the activity coefficients from VLE data, the performance of both methods is similar. On the phase compositions from LLE data, HANNA is slightly less accurate. However, the number of quaternary systems within the mod. UNIFAC horizon is only a fraction of that for the binary and ternary data and the data only covers a small chemical space. Therefore, the results for quaternary systems shown in Fig. S.6 give no quantitative evidence for the superiority of either method.

### 4.3 Predictions for systems containing ionic liquids

Fig. S.7 compares the ACI and LLE predictions of HANNA for systems containing ionic liquids to those of mod. UNIFAC. A system was selected only if the SMILES of at least one of the components contained the following characters: '+' - a positive charge, corresponding to the cation; '-', a negative charge corresponding to the anion; '.', the SMILES notation of the "non-bond" that separates the cation and anion.

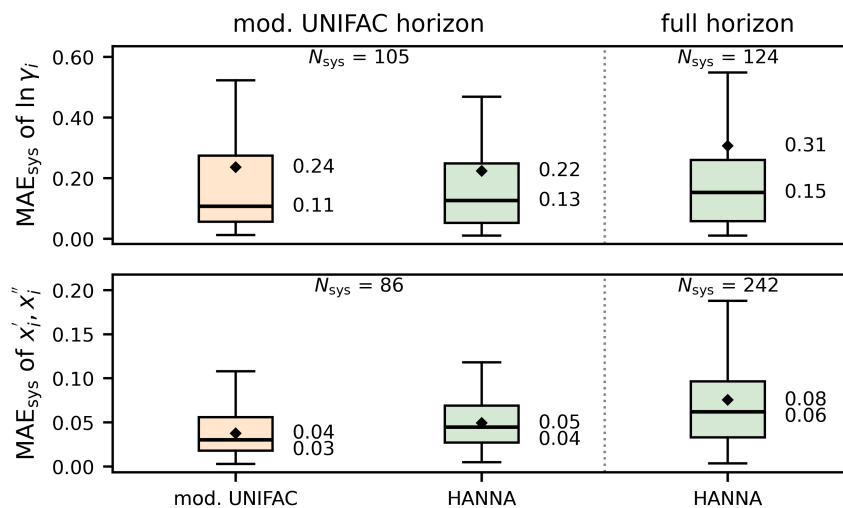

Figure S.6: Boxplots comparing the performance of HANNA for predicting activity coefficients in quaternary VLE (top) and LLE phase compositions (bottom) with that of mod. UNIFAC in terms of the system-wise mean absolute error  $MAE_{sys}$  in  $\gamma_i$  (VLE) or phase compositions  $x'_i$  and  $x''_i$  (LLE). For a fair comparison, HANNA was also evaluated only on those systems for which mod. UNIFAC is applicable (mod. UNIFAC horizon).  $N_{sys}$  denotes the number of test systems within the respective horizon and data type. The boxes represent interquartile ranges and the whiskers are 1.5 times the interquartile range. Diamonds mark the mean, horizontal lines the median of the  $MAE_{sys}$  values.

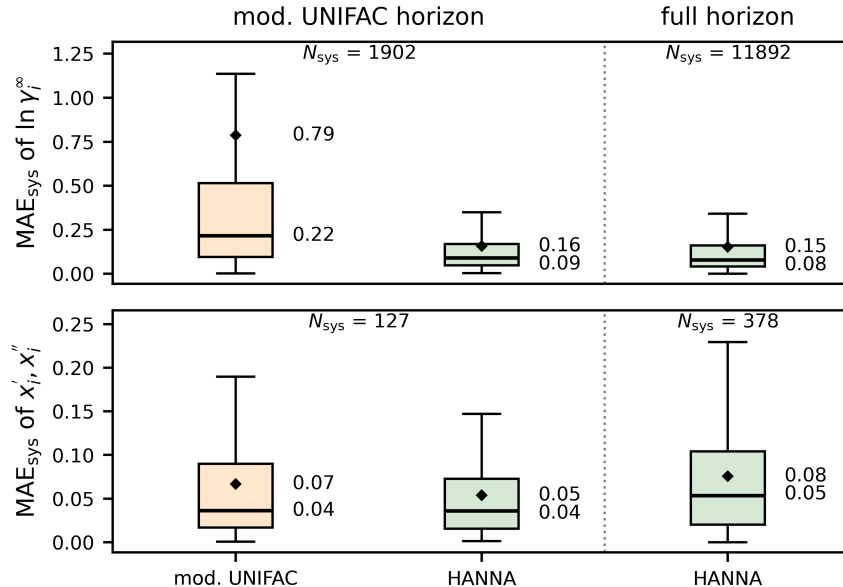

Figure S.7: Boxplots comparing the performance of HANNA for predicting binary ACI (top), and LLE phase compositions (bottom) that include at least one ionic liquid component with that of mod. UNIFAC in terms of the system-wise mean absolute error  $MAE_{sys}$  in  $\gamma_i^\infty$  (ACI) or phase compositions  $x'_i$  and  $x''_i$  (LLE). For a fair comparison, HANNA was also evaluated only on those systems for which mod. UNIFAC is applicable (mod. UNIFAC horizon).  $N_{sys}$  denotes the number of test systems within the respective horizon and data type. The boxes represent interquartile ranges and the whiskers are 1.5 times the interquartile range. Diamonds mark the mean, horizontal lines the median of the  $MAE_{sys}$  values.

#### 4.4 Comparison of HANNA to mod. UNIFAC 2.0

In Figs. S.8, S.9, S.10 HANNA is compared to mod. UNIFAC 2.0 [2] on binary, ternary and quaternary data, respectively. Note that the training of mod. UNIFAC 2.0 did not include any LLE data, however, the training involved data for the excess enthalpy.

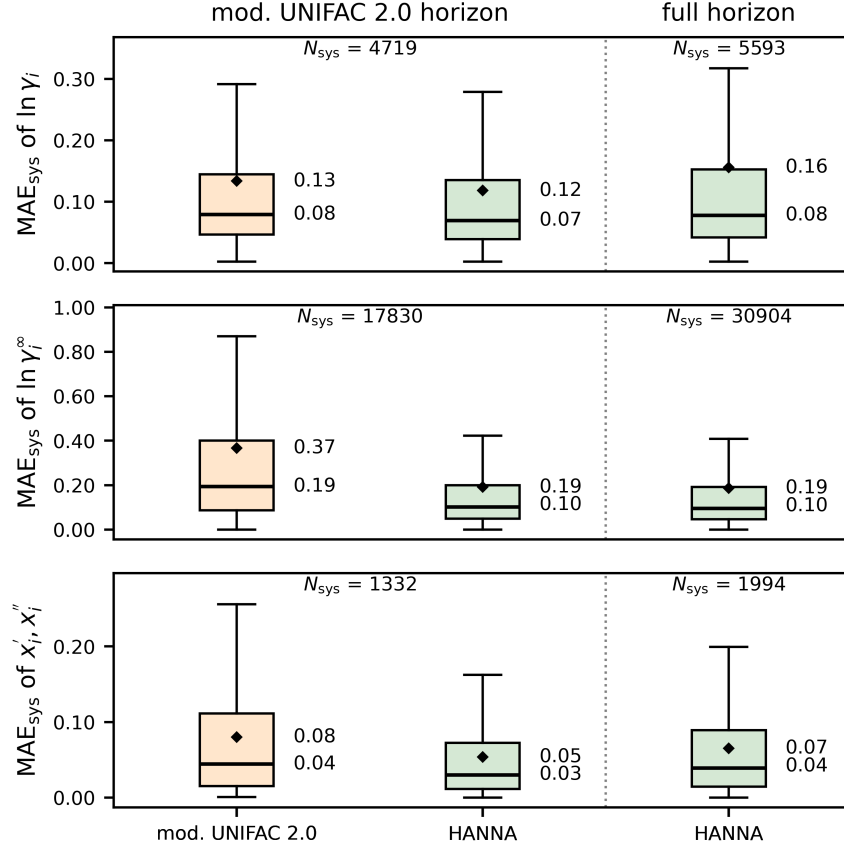

Figure S.8: Boxplots comparing the performance of HANNA for predicting activity coefficients in binary VLE (top), ACI (middle), and LLE phase compositions (bottom) with that of mod. UNIFAC 2.0 [2] in terms of the system-wise mean absolute error MAE<sub>sys</sub> in  $\gamma_i$  (VLE, ACI) or phase compositions  $x_i'$  and  $x_i''$  (LLE). For a fair comparison, HANNA was also evaluated only on those systems for which mod. UNIFAC is applicable (mod. UNIFAC horizon).  $N_{\text{sys}}$  denotes the number of test systems within the respective horizon and data type. The boxes represent interquartile ranges and the whiskers are 1.5 times the interquartile range. Diamonds mark the mean, horizontal lines the median of the MAE<sub>sys</sub> values.



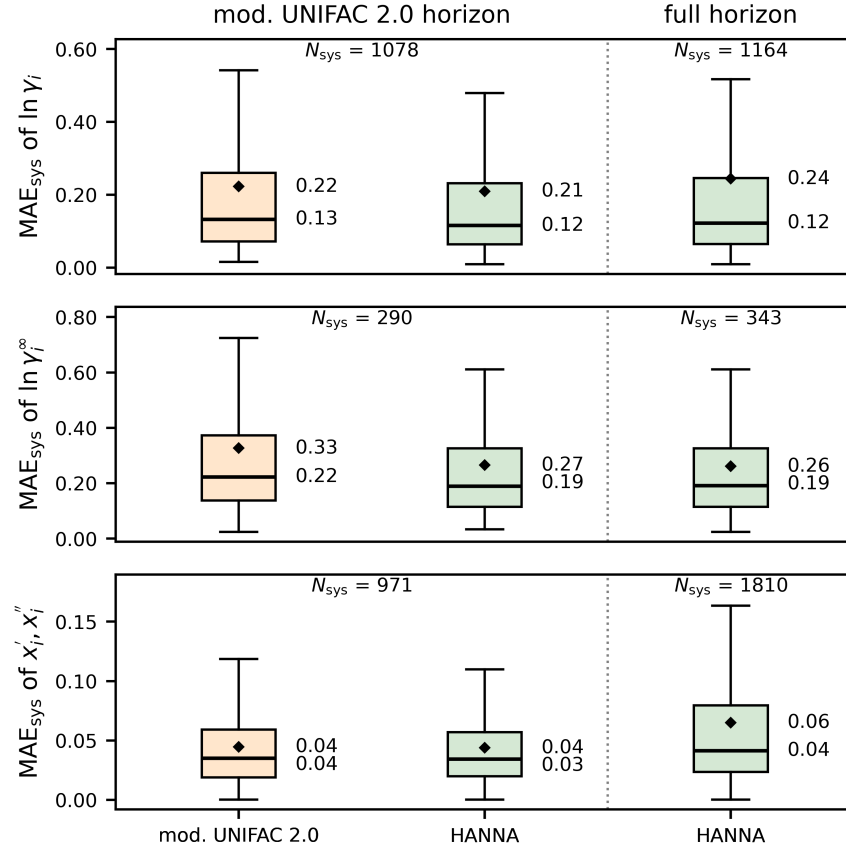

Figure S.9: Boxplots comparing the performance of HANNA for predicting activity coefficients in ternary VLE (top), ACI (middle), and LLE phase compositions (bottom) with that of mod. UNIFAC 2.0 [2] in terms of the system-wise mean absolute error  $\text{MAE}_{\text{sys}}$  in  $\gamma_i$  (VLE, ACI) or phase compositions  $x_i'$  and  $x_i''$  (LLE). For a fair comparison, HANNA was also evaluated only on those systems for which mod. UNIFAC is applicable (mod. UNIFAC horizon).  $N_{\text{sys}}$  denotes the number of test systems within the respective horizon and data type. The boxes represent interquartile ranges and the whiskers are 1.5 times the interquartile range. Diamonds mark the mean, horizontal lines the median of the  $\text{MAE}_{\text{sys}}$  values.

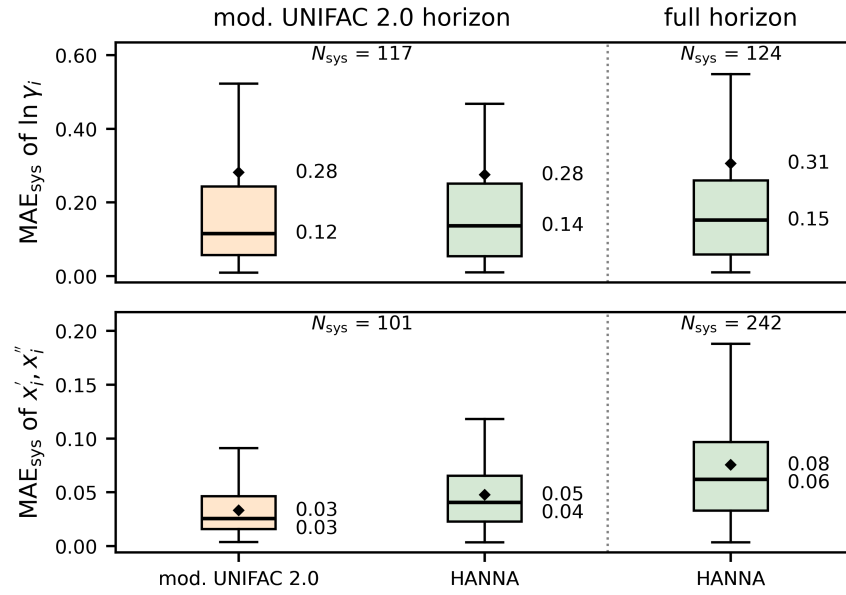

Figure S.10: Boxplots comparing the performance of HANNA for predicting activity coefficients in quaternary VLE (top) and LLE phase compositions (bottom) with that of mod. UNIFAC 2.0 [2] in terms of the system-wise mean absolute error  $\text{MAE}_{\text{sys}}$  in  $\gamma_i$  (VLE) or phase compositions  $x'_i$  and  $x''_i$  (LLE). For a fair comparison, HANNA was also evaluated only on those systems for which mod. UNIFAC is applicable (mod. UNIFAC horizon).  $N_{\text{sys}}$  denotes the number of test systems within the respective horizon and data type. The boxes represent interquartile ranges and the whiskers are 1.5 times the interquartile range. Diamonds mark the mean, horizontal lines the median of the  $\text{MAE}_{\text{sys}}$  values.

#### 4.5 Comparison of HANNA to UNIFAC-LLE

In Figs. S.11, S.12, S.13 HANNA is compared to UNIFAC-LLE [3] on binary, ternary and quaternary LLE data, respectively. Note that UNIFAC-LLE is a parameterization that is only designed for the prediction of LLE in a temperature range of 283.15 K and 313.15 K and therefore no comparison on the VLE or ACI data sets were performed. Consequently, the comparison on the UNIFAC-LLE horizon only includes data points in the respective temperature range. Furthermore, UNIFAC-LLE also included ternary LLE data in the training, resulting in an additional positive bias for UNIFAC-LLE for the ternary and quaternary data.

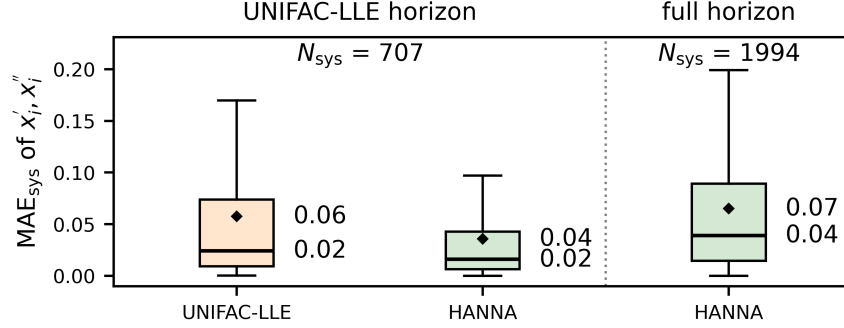

Figure S.11: Boxplots comparing the performance of HANNA for predicting binary LLE phase compositions with that of UNIFAC-LLE [3] in terms of the system-wise mean absolute error  $MAE_{sys}$  in  $x'_i$  and  $x''_i$ . For a fair comparison, HANNA was also evaluated only on those systems and in the temperature range (283.15 K and 313.15 K) for which UNIFAC-LLE is applicable (UNIFAC-LLE horizon).  $N_{sys}$  denotes the number of test systems within the respective horizon and data type. The boxes represent interquartile ranges and the whiskers are 1.5 times the interquartile range. Diamonds mark the mean, horizontal lines the median of the  $MAE_{sys}$  values.

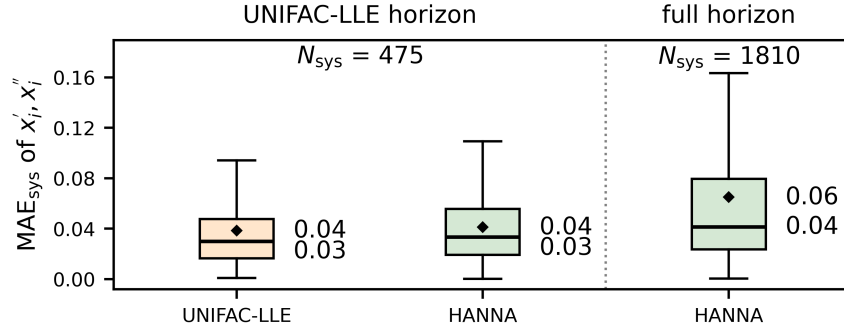

Figure S.12: Boxplots comparing the performance of HANNA for predicting ternary LLE phase compositions with that of UNIFAC-LLE [3] in terms of the system-wise mean absolute error  $MAE_{sys}$  in  $x'_i$  and  $x''_i$ . For a fair comparison, HANNA was also evaluated only on those systems and in the temperature range (283.15 K and 313.15 K) for which UNIFAC-LLE is applicable (UNIFAC-LLE horizon).  $N_{sys}$  denotes the number of test systems within the respective horizon and data type. The boxes represent interquartile ranges and the whiskers are 1.5 times the interquartile range. Diamonds mark the mean, horizontal lines the median of the  $MAE_{sys}$  values.

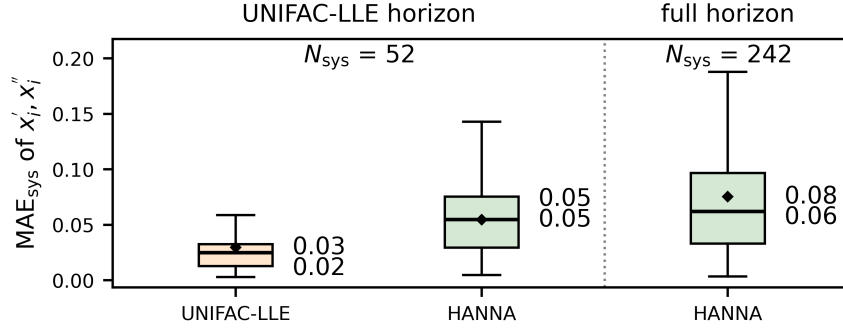

Figure S.13: Boxplots comparing the performance of HANNA for predicting quaternary LLE phase compositions with that of UNIFAC-LLE [3] in terms of the system-wise mean absolute error  $\text{MAE}_{\text{sys}}$  in  $x'_i$  and  $x''_i$ . For a fair comparison, HANNA was also evaluated only on those systems and in the temperature range (283.15 K and 313.15 K) for which UNIFAC-LLE is applicable (UNIFAC-LLE horizon).  $N_{\text{sys}}$  denotes the number of test systems within the respective horizon and data type. The boxes represent interquartile ranges and the whiskers are 1.5 times the interquartile range. Diamonds mark the mean, horizontal lines the median of the  $\text{MAE}_{\text{sys}}$  values.

## 5 Evaluation of the Projection Quality to Multi-Component Systems

Figs. S.14 and S.15 show a comparison of the extrapolation capabilities of HANNA using the geometric projection method of Muggianu [4] to the extrapolation of the most used  $g^E$  models UNIQUAC [5] and NRTL [6] on ternary VLE data. For this purpose, we fitted the respective parameters of the  $g^E$  models ( $\Delta u_{ij}, \Delta u_{ji}$  for UNIQUAC;  $\alpha, A_{ij}, A_{ji}$  for NRTL) for each binary subsystem of a ternary VLE on the predictions of HANNA. This approach ensures that we have an identical description of the ternary mixture in the binary subsystems and only compare the differences arising from their extrapolation behavior going from binary to ternary mixtures. We found that our simple geometric method shows better or similar performance in extrapolation capabilities than both UNIQUAC and NRTL on the considered systems. The improvement is most relevant for the ACI data.

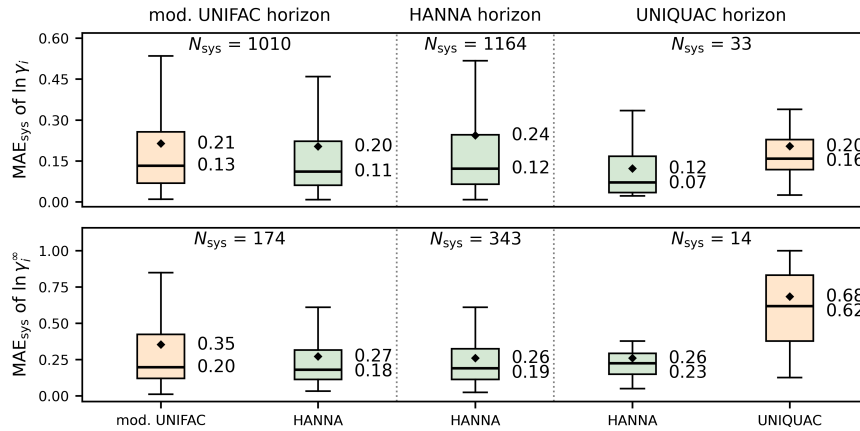

Figure S.14: Boxplots comparing the accuracy of UNIQUAC [5] in extrapolation on activity coefficients derived from ternary VLE (top) and ACI (bottom) data with that of HANNA and mod. UNIFAC. The UNIQUAC predictions for a ternary mixture were obtained by first fitting the parameters  $\Delta u_{ij}$  and  $\Delta u_{ji}$  of the three binary subsystems to predictions of the logarithmic activity coefficients with HANNA. The UNIQUAC horizon only comprises systems for which this fit succeeded and the mean deviation of  $\ln \gamma_i$  lies below 10 %.  $N_{\text{sys}}$  denotes the number of test systems within the respective horizon and data type. The boxes represent interquartile ranges and the whiskers are 1.5 times the interquartile range. Diamonds mark the mean, horizontal lines the median of the  $\text{MAE}_{\text{sys}}$  values.

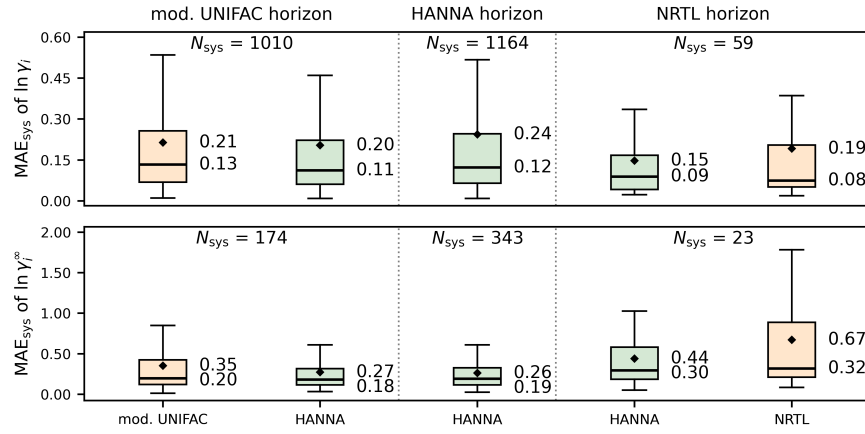

Figure S.15: Boxplots comparing the accuracy of NRTL [6] in extrapolation on ternary VLE (top) and ACI (bottom) data with that of HANNA and mod. UNIFAC. The NRTL predictions for a ternary mixture were obtained by first fitting the parameters  $\alpha$ ,  $A_{ij}$  and  $A_{ji}$  of the three binary subsystems to predictions of the logarithmic activity coefficients with HANNA. The NRTL horizon only comprises systems for which this fit succeeded and the mean deviation of  $\ln \gamma_i$  lies below 10 %.  $N_{\text{sys}}$  denotes the number of test systems within the respective horizon and data type. The boxes represent interquartile ranges and the whiskers are 1.5 times the interquartile range. Diamonds mark the mean, horizontal lines the median of the  $\text{MAE}_{\text{sys}}$  values.

## References

- [1] Thomas Specht, Mayank Nagda, Sophie Fellenz, Stephan Mandt, Hans Hasse, and Fabian Jirasek. Hanna: hard-constraint neural network for consistent activity coefficient prediction. *Chemical Science*, 15(47):19777–19786, 2024.
- [2] Nicolas Hayer, Hans Hasse, and Fabian Jirasek. Modified unifac 2.0-a group-contribution method completed with machine learning. *Industrial & Engineering Chemistry Research*, 64(20):10304–10313, May 2025.
- [3] Thomas Magnussen, Peter Rasmussen, and Aage Fredenslund. Unifac parameter table for prediction of liquid-liquid equilibria. *Industrial & Engineering Chemistry Process Design and Development*, 20(2):331–339, April 1981.
- [4] Yves-Marie Muggianu, Michèle Gambino, and Jean-Pierre Bros. Enthalpies de formation des alliages liquides bismuth-étain-gallium à 723 k. choix d’une représentation analytique des grandeurs d’excès intégrales et partielles de mélange. *Journal de Chimie Physique*, 72:83–88, 1975.
- [5] Denis S. Abrams and John M. Prausnitz. Statistical thermodynamics of liquid mixtures: A new expression for the excess gibbs energy of partly or completely miscible systems. *AIChE Journal*, 21(1):116–128, January 1975.
- [6] Henri Renon and J. M. Prausnitz. Local compositions in thermodynamic excess functions for liquid mixtures. *AIChE Journal*, 14(1):135–144, January 1968.
